# Supplementary material for: Phonon-bottleneck enhanced exciton emission in 2D perovskites
Source: arXiv:2312.10688 source file (2023-12-17)
Supplement: Supplementary file 1 [file Supp.pdf]

# Supplementary Information: Phonon-bottleneck enhanced exciton emission in perovskite monolayers

Joshua J. P. Thompson,[1,2,*] Mateusz Dyksik,[3] Paulina Peksa,[3,4] Katarzyna Posmyk,[3,4] Ambjörn Joki,[5] Raul Perea-Causin,[5] Paul Erhart,[5] Michał Baranowski,[3] Maria Antonietta Loi,[6] Paulina Plochocka,[3,4] and Ermin Malic[1]

[1]*Department of Physics, Philipps-Universität Marburg, Renthof 7, 35032 Marburg*

[2]*Department of Materials Science and Metallurgy, University of Cambridge, Cambridge CB3 0FS, United Kingdom*

[3]*Department of Experimental Physics, Faculty of Fundamental Problems of Technology, Wroclaw University of Science and Technology, 50-370 Wroclaw, Poland*

[4]*Laboratoire National des Champs Magnetiques Intenses, 143 Avenue de Rangueil 31400 Toulouse, France*

[5]*Department of Physics, Chalmers University of Technology, Gothenburg 412 96, Sweden*

[6]*Zernike Institute for Advanced Materials, University of Groningen, Nijenborgh 4, 9747 AG Groningen, The Netherlands*

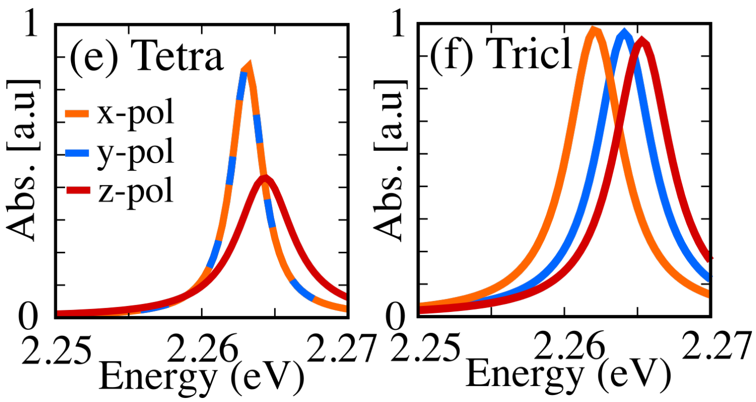


Figure S1: Absorption spectra for an (a) orthorhombic and (b) triclinic perovskite monolayer at 30 K for different polarisations.

## I. ORHTORHOMBIC VS TRICLINIC STRUCTURE

In perovskites, crystal distortion can lead to the material adopting a triclinic rather than orthorhombic phase, leading to a symmetry breaking. The latter is due to small differences in the perovskite crystal lattice in the x and y direction [1–3]. As a result, the exchange interaction along x and y is slightly modified, leading to a distinct optical response, cf. Fig. S1. We find an energy splitting between the x- and y-polarised absorption peaks in the triclnic phase (Fig. **??**b) corresponding to distinct excitonic states. This splitting has little effect on the exciton dynamics and optics in perovskite monolayers, as the bright-dark splitting is an order of magnitude larger [4], and more pronounced effects can be generated with a magnetic field. Therefore in the main text, we neglected the in-plane exciton states splitting seen in some samples [2, 3].

* joshua.thompson@physik.uni-marburg.de

## II. EXPERIMENTAL ANALYSIS

In Fig. S2 we present the temperature evolution of both X$_D$ (dark exciton, Fig. S2a) and X$_B$ (bright exciton, Fig. S2b). Both these emissions blueshift with increasing temperature. The temperature-induced blueshift is simliar for both emission as presented in Fig. S2c.

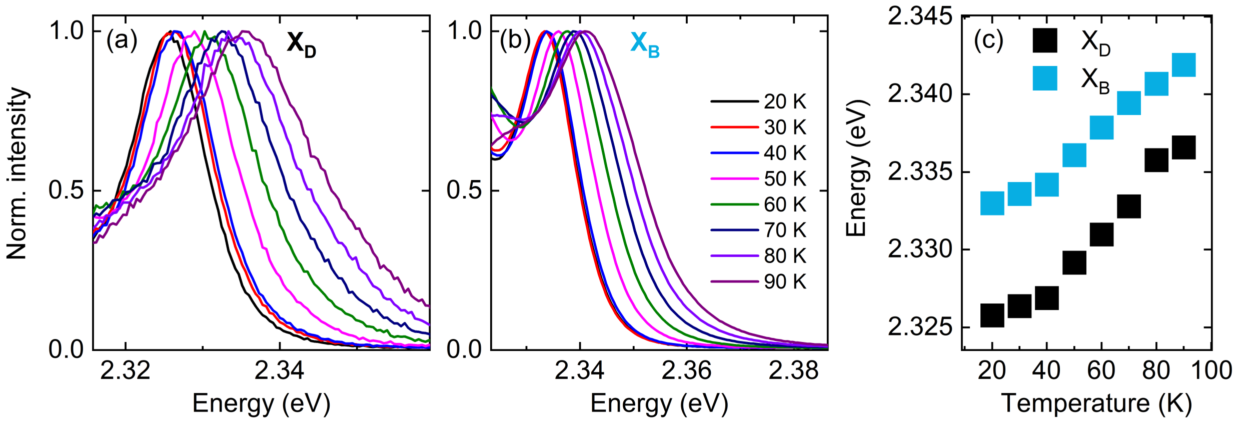


Figure S2: The photoluminescence of (a) dark exciton and (b) bright exciton measured for different sample temperatures. The spectra in panel (a) measured at $B = 60\,\text{T}$. In panel (c) the peak energy of both emissions is presented.

In order to determine the relative intensity of dark (X$_D$) and bright (X$_B$) excitons, the PL spectra is fitted with Gaussian-profiled lineshape. In Fig. S3 the result of such a fitting procedure is presented on the data measured at T=20 K for several magnetic field strenghts. The datapoints represent the experimental data, whereas the fitting componenets are plotted with lines. The blue and black solid lines stand for bright and dark exciton contributions, respectively. The X$_B$ excitonic emission is accompanied by a satellite peak on the low energy side (gray dotted line). This low-energy emission is usually understood as phonon replica/polaronic signal [cite] and its contribution to the PL response surpasses the contribution of the bright state in 0 T (Fig. S3. At higher magnetic field B>25 T an additional componenet (gray dash-dot line) appears at lower energies (≈2.3 eV). This component behaves in the same manner as the brightened X$_D$ thus we assign it to the phonon replica of X$_D$. In all the spectra an additional component is added (dashed gray line) to mitigate the broad background. The brightened X$_D$ dominates over all contributions already at the magnetic field $> 25\,\text{T}$.

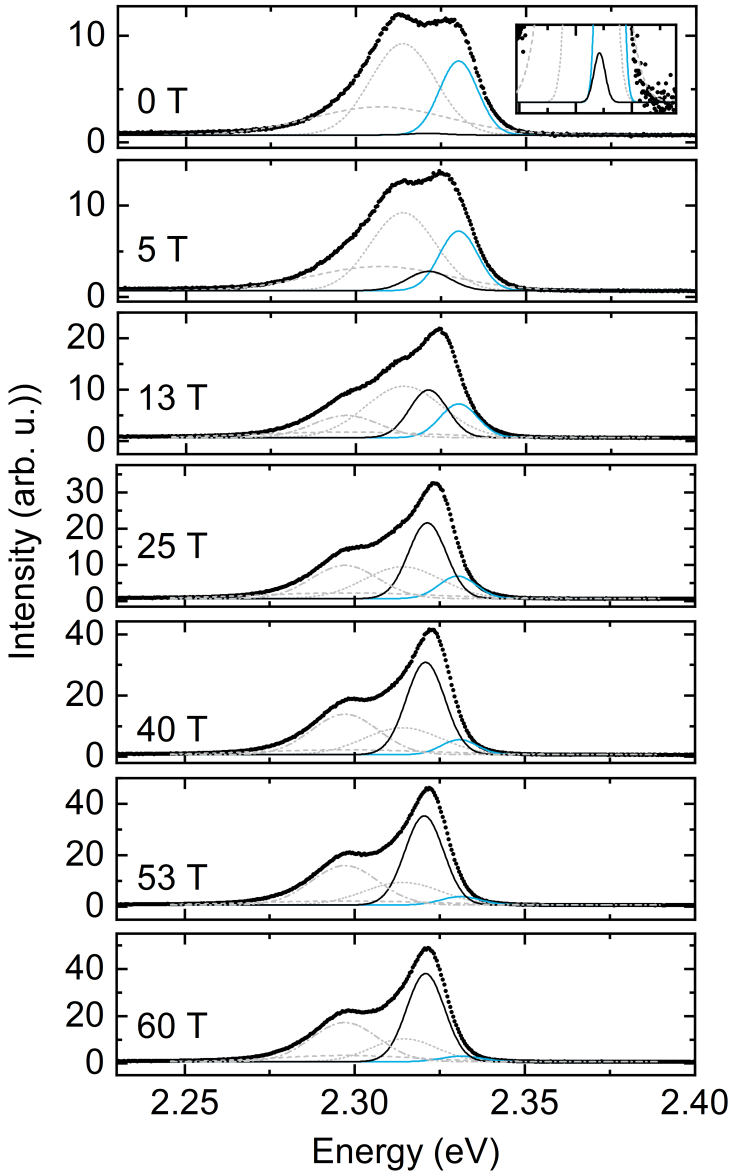


Figure S3: Photoluminescence (PL) spectra (data points) measured at different magnetic fields (T=20 K). In order to reproduce the PL spectra in the whole range of magnetic fields five Gaussian-profiled componenets were used. Blue and dark solid lines represent $X_B$ and $X_D$ emissions, respectively. Dotted gray line desribes the localized/polaronic emission [cite]. Dash-dotted gray contribution behaves similar to $X_D$ in the magnetic field thus is understood as a phonon replica. An additional component (dashed gray) mitigates the broad background. Inset shows the non-zero $X_D$ contribution at 0 T

## III. THEORETICAL MODEL

### A. Wannier Equation

To have a microscopic access to excitonic binding energies, $\epsilon_\eta^{\text{b}}$ and wavefunctions, $\varphi_{\boldsymbol{k}}^\eta$, we evaluate the Wannier equation [5, 6]

$$\left(\frac{\hbar^2\boldsymbol{k}^2}{2\mu_r}+E_{\text{Gap}}\right)\varphi_{\boldsymbol{k}}^\eta+\sum_{\boldsymbol{k'}}V_{\text{Kel}}^{\boldsymbol{kk'}}\varphi_{\boldsymbol{k'}}^\eta=\epsilon_\eta^{\text{b}}\varphi_{\boldsymbol{k}}^\eta \tag{1}$$

where $E_{\text{Gap}}$ is the electronic band gap, $\boldsymbol{k}$ the relative momentum, $V_{\text{Kel}}^{\boldsymbol{kk'}}$ the Fourier transform of the 2D Keldysh potential [7], the reduced mass $\mu_r=\left(\frac{1}{m_e}+\frac{1}{m_h}\right)^{-1}$, and the centre-of-mass mass $M=m_e+m_h$ with $m_e=0.19m_0$ and $m_h=0.25m_0$ as the electron and hole effective mass, respectively (with input parameters obtained from a previous joint DFT/experiment study [8]). Finally, the 2D Keldysh potential is defined as $V_{\text{Kel}}^{\boldsymbol{kk}+\boldsymbol{q}}=e_0^2\left(2\varepsilon_0\varepsilon_sL^2|\boldsymbol{q}|\big(1+\frac{d_P\varepsilon_P}{2\varepsilon_s}|\boldsymbol{q}|\big)\right)^{-1}$ with $\varepsilon_s=3.3$ and $\varepsilon_P=6.1$ as the dielectric constant of the organic spacer layer and perovskite slab, respectively [6, 9], while $d_P=0.636$ is the thickness of the perovskite layer.

### B. Exchange matrix element

The exchange Hamiltonian can be written in second quantisation as

$$\hat{\boldsymbol{H}}_{\text{ex}}=\sum_{\substack{\boldsymbol{k_1k_2k_3k_4}\\s_1,s_2,s_3,s_4}}I_{\boldsymbol{k_1k_2k_3k_4}}^{s_1s_2s_3s_4}\hat{\boldsymbol{c}}_{\boldsymbol{k_1}s_1}^\dagger\hat{\boldsymbol{v}}_{\boldsymbol{k_2}s_2}^\dagger\hat{\boldsymbol{c}}_{\boldsymbol{k_3}s_3}\hat{\boldsymbol{v}}_{\boldsymbol{k_4}s_4} \tag{2}$$

where $\hat{\boldsymbol{a}}^{(\dagger)}$ are annihilation (creation) operators in the conduction ($\hat{\boldsymbol{a}}=\hat{\boldsymbol{c}}$ ) and valence ($\hat{\boldsymbol{a}}=\hat{\boldsymbol{v}}$ ) bands. The interaction strength $I_{\boldsymbol{k_1k_2k_3k_4}}^{s_1s_2s_3s_4}=\int drdr'\psi_{\boldsymbol{k_1}s_1}^{\dagger c}(r)\psi_{\boldsymbol{k_2}s_2}^{\dagger v}(r')V(r-r')\psi_{\boldsymbol{k_4}s_4}^{v}(r)\psi_{\boldsymbol{k_3}s_3}^{c}(r')$ we be expressed in terms of Bloch functions in the 2D case

$$I_{\boldsymbol{k_1k_2k_3k_4}}^{s_1s_2s_3s_4}=\int drdr'e^{-i\boldsymbol{k_1r}}u_{\boldsymbol{k_1}s_1}^{c*}(\boldsymbol{r})e^{-i\boldsymbol{k_2r'}}u_{\boldsymbol{k_2}s_2}^{v*}(\boldsymbol{r'})V(r-r')e^{i\boldsymbol{k_4r}}u_{\boldsymbol{k_4}s_4}^{v*}(\boldsymbol{r})e^{i\boldsymbol{k_3r'}}u_{\boldsymbol{k_3}s_3}^{c*}(\boldsymbol{r'}). \tag{3}$$

From here we perform Fourier transform of the Coulomb potential for a slab of a thickness d and find

$$I_{\boldsymbol{k_1k_2k_3k_4}}^{s_1s_2s_3s_4}=\int drdr'\int_{-d/2}^{d/2}dzdz'\sum_{\boldsymbol{q}_{||}}V_{\text{2D}}(\boldsymbol{q}_{||})e^{i\boldsymbol{q}_{||}(\boldsymbol{r}-\boldsymbol{r'})}e^{-|\boldsymbol{q}_{||}||\boldsymbol{z}-\boldsymbol{z'}|} \tag{4}$$

$$e^{-i\boldsymbol{k_1r}}u_{\boldsymbol{k_1}s_1}^{c*}(\boldsymbol{r})e^{-i\boldsymbol{k_2r'}}u_{\boldsymbol{k_2}s_2}^{v*}(\boldsymbol{r'})e^{i\boldsymbol{k_4r}}u_{\boldsymbol{k_4}s_4}^{v*}(\boldsymbol{r})e^{i\boldsymbol{k_3r'}}u_{\boldsymbol{k_3}s_3}^{c*}(\boldsymbol{r'}). \tag{5}$$

The orbital wavefunctions can be be decomposed into their individual contributions, determined by the spin-orbit coupling. The latter leads to a mixing of the orbital composition of the lowest conduction band [10] with momentum $k$, spin $s$ and orbital $P_i$

$$|s,c,k\rangle = -\frac{1}{\sqrt{3}}\left(\sigma_s\,|P_z,s,k\rangle - |P_x,\overline{s},k\rangle - i\sigma_s\,|P_y,\overline{s},k\rangle\right), \tag{6}$$

where $\sigma = \pm 1$ denotes the up/down spin, respectively. Meanwhile there is no mixing of the valence band $S$ orbitals. As a result we arrive at the following integral

$$\begin{aligned}
I^{s_1s_2s_3s_4}_{\boldsymbol{k_3k_4}} &= \sum_{\boldsymbol{q}} V_{\text{2D}}(\boldsymbol{q}) \sum_{\boldsymbol{G}} \delta_{\boldsymbol{k_4}-\boldsymbol{k_1}+\boldsymbol{q},G}\delta_{\boldsymbol{k_3}-\boldsymbol{k_2}-\boldsymbol{q},-G} \int_{-d/2}^{d/2} dz dz' e^{-|\boldsymbol{q}||\boldsymbol{z}-\boldsymbol{z'}|} \\
&\times \frac{1}{\sqrt{3}} \int_{\text{UC}} dr \Big[\sigma_{s_1}\langle P_z, s_1, \boldsymbol{k_4}+\boldsymbol{q}-\boldsymbol{G}| - \langle P_x, \overline{s}_1, \boldsymbol{k_4}+\boldsymbol{q}-\boldsymbol{G}| + i\sigma_{s_1}\langle P_y, \overline{s}_1, \boldsymbol{k_4}+\boldsymbol{q}-\boldsymbol{G}|\Big] \\
&\times e^{i\boldsymbol{Gr}}\,|S, s_4, \boldsymbol{k_4}\rangle \\
&\times \frac{1}{\sqrt{3}} \int_{\text{UC}} dr' \langle S, s_2, \boldsymbol{k_3}-\boldsymbol{q}+\boldsymbol{G}|\, e^{-i\boldsymbol{Gr'}} \\
&\times \Big[\sigma_{s_3}\,|P_z, s_3, \boldsymbol{k_3}\rangle - |P_x, \overline{s}_3, \boldsymbol{k_3}\rangle - i\sigma_{s_3}\,|P_y, \overline{s}_3, \boldsymbol{k_3}\rangle\Big].
\end{aligned}$$

There are two types of interactions that need to be calculated: the long-range interaction with $\boldsymbol{G} = 0$ and the short-range interaction with $\boldsymbol{G} \neq 0$. Furthermore, since only the wavefunction overlap of same-spin states is non-zero, we can split the above integral into two further parts: those that couple along z, and those that couple in the perovskite plane (x and y). In the electronic picture we arrive at the following expression

$$\begin{aligned}
H_{\text{ex-el}} = \frac{1}{3} \sum_{\substack{\boldsymbol{k_3k_4q} \\ s_1,s_2,s_3,s_4}} \Bigg[ &\sum_{\boldsymbol{G}\neq 0} V_{\text{2D}}(\boldsymbol{G})(\delta_{\overline{s_1},s_4}\delta_{\overline{s_3},s_2}\Gamma^{\text{SR}}_{s_1,s_3}(\boldsymbol{G}) + \sigma_{s_1}\sigma_{s_3}\delta_{s_1,s_4}\delta_{s_3,s_2}\Lambda^{k_3,k_4}_{a,d,\text{SR}}(\boldsymbol{G})) \\
&+ V_{\text{2D}}(\boldsymbol{q})(\delta_{\overline{s_1},s_4}\delta_{\overline{s_3},s_2}\Gamma^{\text{LR}}_{s_1,s_3}(\boldsymbol{q}) + \sigma_{s_1}\sigma_{s_3}\delta_{s_1,s_4}\delta_{s_3,s_2}\Lambda^{k_3,k_4}_{\text{LR}}(\boldsymbol{q}))\Bigg] \\
&\times \hat{\boldsymbol{c}}^{\dagger}_{\boldsymbol{k_4}+\boldsymbol{q}s_1}\hat{\boldsymbol{v}}^{\dagger}_{\boldsymbol{k_3}-\boldsymbol{q}s_2}\hat{\boldsymbol{c}}_{\boldsymbol{k_3}s_3}\hat{\boldsymbol{v}}_{\boldsymbol{k_4}s_4} + h.c.
\end{aligned}$$

Here, the first line corresponds to the short-range interaction (reciprocal lattice vector $\boldsymbol{G} \neq 0$) parametrised by the coupling of the same-spin conduction-band $P_z$-orbitals with valence-band $s$-orbitals $\Lambda^{k_3,k_4}_{\text{SR}}(\boldsymbol{G})$ and the coupling of opposite-spin conduction-band $P_{x/y}$-orbitals with valence-band $S$-orbitals $\Gamma^{k_3,k_4}_{\text{SR}}(\boldsymbol{G})$. The second line corresponds to the long-range interaction, corresponding to small momentum transfer within the first Brillouin zone, and parameterised in the same way by $\Lambda^{k_3,k_4}_{\text{LR}}(\boldsymbol{q})$ and $\Gamma^{k_3,k_4}_{\text{LR}}(\boldsymbol{q})$. The spin conservation is described with the Kronecker deltas $\delta_{s_a,s_b}$.

Using the solution to the Wannier equation, we transform this Hamiltonian into the excitonic basis, with exciton annihilation (creation) operators $\hat{\boldsymbol{X}}_{\boldsymbol{q}}^{\nu,s_a,s_b(\dagger)}$

$$H_{\text{ex-X}} = \frac{1}{3} \sum_{\substack{\boldsymbol{k_3 k_4 q} \\ s_1,s_2,s_3,s_4}} \Bigg[ \sum_{\boldsymbol{G}\neq 0} V_{\text{2D}}(\boldsymbol{G})(\delta_{\overline{s_1},s_4}\delta_{\overline{s_3},s_2}\Gamma^{\text{SR}}_{s_1,s_3}(\boldsymbol{G}) + \sigma_{s_1}\sigma_{s_3}\delta_{s_1,s_4}\delta_{s_3,s_2}\Lambda^{k_3,k_4}_{\text{SR}}(\boldsymbol{G}))$$
$$+ V_{\text{2D}}(\boldsymbol{q})(\delta_{\overline{s_1},s_4}\delta_{\overline{s_3},s_2}\Gamma^{\text{LR}}_{s_1,s_3}(\boldsymbol{q}) + \sigma_{s_1}\sigma_{s_3}\delta_{s_1,s_4}\delta_{s_3,s_2}\Lambda^{k_3,k_4}_{\text{LR}}(\boldsymbol{q}))\Bigg]$$
$$\times \sum_{\mu\nu} \varphi^{\nu}_{\boldsymbol{k_4}+\beta\boldsymbol{q}}\varphi^{\mu *}_{\boldsymbol{k_3}-\alpha\boldsymbol{q}}\hat{\boldsymbol{X}}_{\boldsymbol{q}}^{\nu,s_1,s_4\dagger}\hat{\boldsymbol{X}}_{\boldsymbol{q}}^{\mu,s_3,s_2}.$$

In order to derive the exciton fine-structure, we note that we transform the Hamiltonian into a new spin-hybridised basis. Assuming only the lowest energy excitons are relevant $\mu = \nu = 1s$ we write

$$\hat{\boldsymbol{X}}_{\boldsymbol{q}}^{s_1,s_4} = \sum_n D_{\boldsymbol{q}}^{s_1,s_4,n,*}\hat{\boldsymbol{Y}}_{\boldsymbol{q}}^{n}, \tag{7}$$

such that we only have to solve the eigenvalue equation

$$\frac{1}{3}|\varphi(\boldsymbol{r}=0)|^2 \begin{pmatrix} I_Z & 0 & 0 & -I_Z \\ 0 & I_r^{s_1=\uparrow,s_3=\uparrow} & I_r^{s_1=\downarrow,s_3=\uparrow} & 0 \\ 0 & I_r^{s_1=\uparrow,s_3=\downarrow} & I_r^{s_1=\downarrow,s_3=\downarrow} & 0 \\ -I_Z & 0 & 0 & I_Z \end{pmatrix} \begin{pmatrix} D_{\boldsymbol{q}}^{\uparrow,\uparrow,n} \\ D_{\boldsymbol{q}}^{\uparrow,\downarrow,n} \\ D_{\boldsymbol{q}}^{\downarrow,\uparrow,n} \\ D_{\boldsymbol{q}}^{\downarrow,\downarrow,n} \end{pmatrix} = E_{\boldsymbol{q}}^{n} \begin{pmatrix} D_{\boldsymbol{q}}^{\uparrow,\uparrow,n} \\ D_{\boldsymbol{q}}^{\uparrow,\downarrow,n} \\ D_{\boldsymbol{q}}^{\downarrow,\uparrow,n} \\ D_{\boldsymbol{q}}^{\downarrow,\downarrow,n}, \end{pmatrix} \tag{8}$$

where we define the entries as

$$I_Z(\boldsymbol{q}) = V_{\text{2D}}(\boldsymbol{q})\Lambda_{\text{LR}}(\boldsymbol{q}) + \sum_{\boldsymbol{G}\neq 0} V_{\text{2D}}(\boldsymbol{G})\Lambda_{\text{SR}}(\boldsymbol{G}))$$
$$I_r^{ss'}(\boldsymbol{q}) = V_{\text{2D}}(\boldsymbol{q})\Gamma^{\text{LR}}_{s,s'}(\boldsymbol{q}) + \sum_{\boldsymbol{G}\neq 0} V_{\text{2D}}(\boldsymbol{G})\Gamma^{\text{SR}}_{s,s'}(\boldsymbol{G}).$$

In the orthorombic phase, with $D_{4h}$ symmetry $I_r^{s_1=\uparrow,s_3=\uparrow} = I_r^{s_1=\downarrow,s_3=\downarrow}$ and off digaonal terms $I_r^{s_1=\downarrow,s_3=\uparrow}$ and $I_r^{s_1=\uparrow,s_3=\downarrow}$ vanish. Important to note is the the first terms in these equations, corresponding to the long-range interaction, vanish at $\boldsymbol{q} = 0$, which is consistent with previous calculations. The $\boldsymbol{q}$-dependence, however, shifts the excitonic dispersion from a parabolic towards a more linear branch. However, due to screening at large $\boldsymbol{q}$, the effect is only visible at small $\boldsymbol{q}$ [11, 12],

and has little effect on the exciton dynamics. The resulting excitonic energy levels are then

$$E_{\boldsymbol{q}}^{n=0} = \frac{\hbar^2 \boldsymbol{q}^2}{2M} + \epsilon_{1s}^{\mathrm{b}},$$
$$E_{\boldsymbol{q}}^{n=1} = \frac{2}{3}|\varphi(\boldsymbol{r}=0)|^2 I_Z(\boldsymbol{q}) + \frac{\hbar^2 \boldsymbol{q}^2}{2M} + \epsilon_{1s}^{\mathrm{b}},$$
$$E_{\boldsymbol{q}}^{n=2} = \frac{1}{3}|\varphi(\boldsymbol{r}=0)|^2 I_r^{\uparrow\uparrow}(\boldsymbol{q}) + \frac{\hbar^2 \boldsymbol{q}^2}{2M} + \epsilon_{1s}^{\mathrm{b}},$$
$$E_{\boldsymbol{q}}^{n=3} = \frac{1}{3}|\varphi(\boldsymbol{r}=0)|^2 I_r^{\uparrow\uparrow}(\boldsymbol{q}) + \frac{\hbar^2 \boldsymbol{q}^2}{2M} + \epsilon_{1s}^{\mathrm{b}}.$$

In the case of a triclinic crystal, the off-diagonal terms $I_r^{s_1=\uparrow,s_3=\downarrow}$ and $I_r^{s_1=\downarrow,s_3=\uparrow}$ are also non-zero. However, in real systems the asymmetry is small ($< 1\%$) [1] and hence only leads to a small splitting between the resulting eigenstates and does not profoundly change the emergence of a phonon-bottleneck. The splitting is typically of the order of 1-2 meV [3]. The parameterisation of this Hamiltonian is challenging since the short-range terms include an infinite summation, however it is possible to use either DFT [11] or experimental comparison [13] to estimate these parameters.

We include the in-plane magnetic field, $B$, focusing only on the 1s state

$$H_{X-\mathrm{Mag}} = \sum_{\boldsymbol{q}} \sum_{s_1,s_2,s_3,s_4} \left( g_{\mathrm{mag}}^c \delta_{\overline{s_1},s_3} \delta_{s_2,s_4} - g_{\mathrm{mag}}^v \delta_{s_1,s_3} \delta_{\overline{s_2},s_4} \right) X_{\boldsymbol{q}}^{s_1 s_4 \dagger} X_{\boldsymbol{q}}^{s_3 s_2} \tag{9}$$

such that $g_{\mathrm{mag}}^{c/v}(B) = g^{c/v} \frac{\mu_B B}{2}$, where $g^{c/v}$ are the g-factors in the excitonic basis. The exchange eigenproblem in this case becomes modified, with extra terms coupling single-spin flips

$$\begin{pmatrix} I_Z & -g_{\mathrm{mag}}^v(B) & g_{\mathrm{mag}}^c(B) & -I_Z \\ -g_{\mathrm{mag}}^v(B) & I_r^{s_1=\uparrow,s_3=\uparrow} & I_r^{s_1=\downarrow,s_3=\uparrow} & g_{\mathrm{mag}}^c(B) \\ g_{\mathrm{mag}}^c(B) & I_r^{s_1=\uparrow,s_3=\downarrow} & I_r^{s_1=\uparrow,s_3=\uparrow} & -g_{\mathrm{mag}}^v(B) \\ -I_Z & g_{\mathrm{mag}}^c(B) & -g_{\mathrm{mag}}^v(B) & I_Z \end{pmatrix} \begin{pmatrix} D_{\boldsymbol{q}}^{\uparrow,\uparrow,n}(B) \\ D_{\boldsymbol{q}}^{\uparrow,\downarrow,n}(B) \\ D_{\boldsymbol{q}}^{\downarrow,\uparrow,n}(B) \\ D_{\boldsymbol{q}}^{\downarrow,\downarrow,n}(B) \end{pmatrix} = E_{\boldsymbol{q}}^n(B) \begin{pmatrix} D_{\boldsymbol{q}}^{\uparrow,\uparrow,n}(B) \\ D_{\boldsymbol{q}}^{\uparrow,\downarrow,n}(B) \\ D_{\boldsymbol{q}}^{\downarrow,\uparrow,n}(B) \\ D_{\boldsymbol{q}}^{\downarrow,\downarrow,n}(B) \end{pmatrix}, \tag{10}$$

absorbing the factor $\frac{1}{3}|\varphi(\boldsymbol{r}=0)|^2$ into $I_r$ and $I_Z$

The characterisation of these excitonic states is determined by their optical behaviour (bright, dark, gray). To this end, we examine the optical matrix element

$$|M_\sigma^n(B)|^2 \propto |\psi^{1s}(\boldsymbol{r}=0)|^2 |\boldsymbol{e}_\sigma \cdot \sum_{ss'} d_{cv}^{ss'} D_0^{ss'n}(B)|^2 \tag{11}$$

where $|\psi^{1s}(\boldsymbol{r}=0)|^2 = |\sum_k \varphi_{\boldsymbol{k}}^{1s}|^2$ describes the probability of the constituent electron and hole being located at the same point, $\boldsymbol{e}_\sigma$ is the polarisation Jones vector of the incoming light, and $d_{cv}^{ss'}$ are the transition dipoles between spin-bands with $s$ and $s'$.

### C. Exciton-phonon scattering

To calculate the phonon-mediated dynamics, we start with the exciton-phonon Hamiltonian as previous calculated [14]

$$\hat{\boldsymbol{H}}_{\text{X-Ph}} = \sum_{\mu\nu\boldsymbol{Q}\boldsymbol{q}\alpha} \Omega^{s_1 s_4 s_2 s_3}_{\alpha\boldsymbol{q}} X^{s_1 s_4 \dagger}_{\boldsymbol{Q}+\boldsymbol{q}} X^{s_2 s_3}_{\boldsymbol{Q}} \hat{\boldsymbol{b}}^{\alpha}_{\boldsymbol{q}} + h.c \tag{12}$$

We then perform a transformation into the exchange basis

$$\hat{\boldsymbol{H}}_{\text{X-Ph}} = \sum_{\mu\nu\boldsymbol{Q}\boldsymbol{q}\alpha} \sum_{n,n'} \Omega^{n'n}_{\alpha\boldsymbol{q}} Y^{n\dagger}_{\boldsymbol{Q}+\boldsymbol{q}} Y^{n'}_{\boldsymbol{Q}} \hat{\boldsymbol{b}}^{\alpha}_{\boldsymbol{q}} + h.c, \tag{13}$$

where $\Omega^{n'n}_{\alpha\boldsymbol{q}} = \sum_{s,s',s''} \left( G^{\text{elec},\alpha,s,s'\boldsymbol{q}*} D^{ss''n}_{\boldsymbol{q}} D^{s's''n'*}_{\boldsymbol{q}} - \delta_{s,s'} G^{\text{hole},\alpha,s,s'\boldsymbol{q}} D^{s''sn}_{\boldsymbol{q}} D^{s''sn'*}_{\boldsymbol{q}} \right)$. The strengths of the exciton-phonon scattering, $G^{\text{elec}}$ and hole, $G^{\text{hole}}$, are determined as follows

$$G^{\text{elec},\alpha,s,s'\boldsymbol{q}*} = g^{c,\alpha,s,s'\boldsymbol{q}}_{\text{ph}} \mathcal{F}(\beta\boldsymbol{q}), \quad G^{\text{hole},\alpha,s,s'\boldsymbol{q}*} = g^{v,\alpha,s,s'\boldsymbol{q}}_{\text{ph}} \mathcal{F}(-\varrho\boldsymbol{q}) \tag{14}$$

with the form factors $\mathcal{F}(\boldsymbol{q}) = \sum_{\boldsymbol{k}} \varphi^*_{\boldsymbol{k}} \varphi_{\boldsymbol{k}+\boldsymbol{q}}$. The constants $g^{c(v),\alpha,s,s'\boldsymbol{q}}_{\text{ph}}$ describe the electron-phonon coupling in the conduction (valence) bands, which we obtain using a deformation potential model [6].

The exciton dynamics can be calculated by solving a series of semiconductor Bloch equations [14, 15]. We use Heisenberg's equation of motion, $\partial_t N^n_{\boldsymbol{Q}} = -i\hbar \left\langle [N^n_{\boldsymbol{Q}}, \hat{\boldsymbol{H}}_X] \right\rangle$ to derive these equations, using the Markov and cluster expansion approximation [15] to truncate these equations to the most important terms. Finally, we find for the exciton occupation

$$\partial_t N^n_{\boldsymbol{Q}} = \sum_{n'\boldsymbol{Q'}} \left( W^{n'n}_{\boldsymbol{Q'}\boldsymbol{Q}} N^{n'}_{\boldsymbol{Q'}} - W^{nn'}_{\boldsymbol{Q}\boldsymbol{Q'}} N^n_{\boldsymbol{Q}} \right), \tag{15}$$

where the scattering strength from exciton energy level $n$ and momentum $\boldsymbol{Q}$ to level $n'$ and momentum $\boldsymbol{Q'}$ is defined by $W^{nn'}_{\boldsymbol{Q}\boldsymbol{Q'}}$. This has the form

$$W^{nn'}_{\boldsymbol{Q}\boldsymbol{Q'}} = \frac{2\pi}{\hbar} \sum_{\alpha\pm} |\Omega^{nn'}_{\alpha\boldsymbol{Q'}-\boldsymbol{Q}}|^2 \left( \frac{1}{2} \pm \frac{1}{2} + n_{\alpha\boldsymbol{Q'}-\boldsymbol{Q}} \right) \delta\Big( E^{n'}_{\boldsymbol{Q'}} - E^n_{\boldsymbol{Q}} + \hbar\Omega^{\alpha}_{\boldsymbol{Q'}-\boldsymbol{Q}} \Big) \tag{16}$$

where the sum over $\pm$ corresponds to absorption/emission of phonons and where $n_{\alpha\boldsymbol{q}}$ denotes the population of phonons in the mode $\alpha$ and momentum $\boldsymbol{q}$. The corresponding phonon energy is $\hbar\Omega^{\alpha}_{\boldsymbol{q}}$. The delta function ensures energy conservation in the process. We include both acoustic and optical modes [6], with the latter being especially crucial for scattering between bright and dark states. Importantly, the mixing of conduction band spins due to spin-orbit coupling relaxes the

strict spin conservation. This process is known as the Elliott-Yafet mechanism, a common source of spin-depolarisation in systems with a strong spin-orbit coupling. In this system, this process is necessary to enable phonon-scattering between the bright and dark/gray excitons.

### D. Exction optics and linewidth

The exciton absorption can be described using the Elliot formula, which depends on the magnetic field and temperature is

$$I^{\sigma}_{\text{Abs}}(B,T) \propto \Im\left(\sum_{n} \frac{|M^n_{\sigma}(B)|^2}{\hbar\omega - E^n_{\boldsymbol{q}=0}(B) + i\gamma(B,T)}\right) \tag{17}$$

with the linewidth $\gamma$ and optical energy and polarisation defined as $\hbar\omega$ and $\sigma$, respectively. The time-resolved PL can be calculated with

$$I^{\sigma}_{\text{PL}}(B,T,t) \propto \Im\left(\sum_{n} \frac{N^n_{\boldsymbol{Q}=0}(B,T,t)|M^n_{\sigma}(B)|^2}{\hbar\omega - E^n_{\boldsymbol{q}=0}(B) + i\gamma(B,T)}\right) \tag{18}$$

which differs from the absorption due to the temporally evolving exciton population, $N^n_{\boldsymbol{Q}=0}(B,T,t)$. The linewidth of exciton resonances can be be calculated microscopically. We consider radiative broadening as well and phonon-induced non-radiative broadening. The radiative coupling can be described as

$$\gamma^n_{\text{rad}}(B) = \frac{\hbar e^2}{2m_0^2\epsilon_0 c_0 n E^n_{\boldsymbol{q}=0}(B)}|M^n_{\sigma}(B)|^2 \tag{19}$$

with the refractive index $n = 1.82$. The radiative coupling depends on the excitonic wavefunctions and the exciton energy and is independent of temperature. The non-radiative decay is determined by

$$\gamma^n_{\text{non-rad}}(B,T) = \pi \sum_{\boldsymbol{q}\alpha\pm} |\Omega^{nn'}_{\alpha\boldsymbol{q}}|^2 \left(\frac{1}{2} \pm \frac{1}{2} + n_{\alpha\boldsymbol{q}}\right) \delta\left(E^{n'}_{\boldsymbol{q}} - E^n_0 \pm \hbar\Omega^{\alpha}_{\boldsymbol{q}}\right), \tag{20}$$

depending on the phonon population $n_{\alpha\boldsymbol{q}}$ in the mode $\alpha$ and momentum $\boldsymbol{q}$. We take into account both phonon absorption and emission processes ($\pm$). The non-radiative broadening is therefore temperature dependent.

---


[1] Fang, H.-H.; Yang, J.; Tao, S.; Adjokatse, S.; Kamminga, M. E.; Ye, J.; Blake, G. R.; Even, J.; Loi, M. A. Unravelling light-induced degradation of layered perovskite crystals and Design of Efficient Encapsulation for improved Photostability. *Advanced Functional Materials* **2018**, *28*, 1800305.

[2] Do, T. T. H.; Granados del Aguila, A.; Zhang, D.; Xing, J.; Liu, S.; Prosnikov, M.; Gao, W.; Chang, K.; Christianen, P. C.; Xiong, Q. Bright exciton fine-structure in two-dimensional lead halide perovskites. *Nano Lett.* **2020**, *20*, 5141–5148.

[3] Posmyk, K.; Zawadzka, N.; Dyksik, M.; Surrente, A.; Maude, D. K.; Kazimierczuk, T.; Babinski, A.; Molas, M. R.; Paritmongkol, W.; Maczka, M.; others Quantification of exciton fine structure splitting in a two-dimensional perovskite compound. *The Journal of Physical Chemistry Letters* **2022**, *13*, 4463–4469.

[4] Dyksik, M.; Duim, H.; Maude, D. K.; Baranowski, M.; Loi, M. A.; Plochocka, P. Brightening of dark excitons in 2D perovskites. *Science advances* **2021**, *7*, eabk0904.

[5] Koch, S.; Kira, M.; Khitrova, G.; Gibbs, H. Semiconductor excitons in new light. *Nature materials* **2006**, *5*, 523–531.

[6] Feldstein, D.; Perea-Causin, R.; Wang, S.; Dyksik, M.; Watanabe, K.; Taniguchi, T.; Plochocka, P.; Malic, E. Microscopic picture of electron–phonon interaction in two-dimensional halide perovskites. *The Journal of Physical Chemistry Letters* **2020**, *11*, 9975–9982.

[7] Keldysh, L. V. Coulomb interaction in thin semiconductor and semimetal films. *Soviet Journal of Experimental and Theoretical Physics Letters* **1979**, *29*, 658.

[8] Ziegler, J. D.; Zipfel, J.; Meisinger, B.; Menahem, M.; Zhu, X.; Taniguchi, T.; Watanabe, K.; Yaffe, O.; Egger, D. A.; Chernikov, A. Fast and anomalous exciton diffusion in two-dimensional hybrid perovskites. *Nano Letters* **2020**, *20*, 6674–6681.

[9] Hong, X.; Ishihara, T.; Nurmikko, A. Dielectric confinement effect on excitons in PbI 4-based layered semiconductors. *Physical Review B* **1992**, *45*, 6961.

[10] Becker, M. A.; Vaxenburg, R.; Nedelcu, G.; Sercel, P. C.; Shabaev, A.; Mehl, M. J.; Michopoulos, J. G.; Lambrakos, S. G.; Bernstein, N.; Lyons, J. L.; others Bright triplet excitons in caesium lead halide perovskites. *Nature* **2018**, *553*, 189–193.

[11] Yu, H.; Liu, G.-B.; Gong, P.; Xu, X.; Yao, W. Dirac cones and Dirac saddle points of bright excitons in monolayer transition metal dichalcogenides. *Nature communications* **2014**, *5*, 3876.

[12] Thompson, J. J.; Brem, S.; Fang, H.; Antón-Solanas, C.; Han, B.; Shan, H.; Dash, S. P.; Wieczorek, W.; Schneider, C.; Malic, E. Valley-exchange coupling probed by angle-resolved photoluminescence. *Nanoscale Horizons* **2022**, *7*, 77–84.

[13] Gramlich, M.; Swift, M. W.; Lampe, C.; Lyons, J. L.; Döblinger, M.; Efros, A. L.; Sercel, P. C.; Urban, A. S. Dark and bright excitons in halide perovskite nanoplatelets. *Advanced Science* **2022**, *9*,

2103013.

[14] Brem, S.; Selig, M.; Berghaeuser, G.; Malic, E. Exciton relaxation cascade in two-dimensional transition metal dichalcogenides. *Scientific reports* **2018**, *8*, 8238.

[15] Kira, M.; Koch, S. W. Many-body correlations and excitonic effects in semiconductor spectroscopy. *Progress in quantum electronics* **2006**, *30*, 155–296.
